# Supplementary material for: Standardization of multivariate Gaussian mixture models and background adjustment of PET images in brain oncology
Source: arXiv:1710.08508 source file (2018-02-13)

Supplementary Materials to "Standardization of multivariate Gaussian mixture models and background adjustment of PET images in brain oncology"

# A Proofs

*Proof of Theorem 2.1.* We first consider the transformation with the hard assignment $T_H$.

Part 1). If $\pi_1 \to 1$, then it follows that $s_1 \xrightarrow{p} 1$, $r(Y) = O_p(1)$ and $\pi_0 \to -\infty$. Therefore, we have $\widetilde{s}_1 = \mathbb{1}(r(Y) > \pi_0) \xrightarrow{p} 1$, and thus $\mathbb{1}(\widetilde{s}_1 = s_1) \xrightarrow{p} 1$. By applying (11), we obtain that $T_H - Z = O_p(1) \cdot \mathbb{1}(\widetilde{s}_1 \neq s_1) = o_p(1)$, which concludes the proof. Similar argument follows when $\pi_2 \to 1$.

Part 2). According to the result in (10), it is easy to obtain that when $s_1 = 1$, $r(Y) \to +\infty$ with probability 1 and when $s_2 = 1$, $r(Y) \to -\infty$ with probability 1. Therefore, when $s_1 = 1$, we have $\widetilde{s}_1 = 1$ with probability 1; when $s_2 = 1$, we have $\widetilde{s}_2 = 1$ with probability 1. Consequently, it follows that $\widetilde{s}_1 - s_1 \xrightarrow{a.s.} 0$ and thus $T_H \xrightarrow{a.s.} Z$ by applying the result in (11).

Part 3) and 4), we obtain that $T_H \xrightarrow{a.s.} Z$ by applying the result in (11) directly.

Then we consider the case when the soft assignment is used, i.e., the transformation $T_S^{(1)}$. Under conditions in part 1) and 2), we note that $w_1(1-w_1) \xrightarrow{a.s.} 0$. This implies the asymptotic equivalence between the soft and hard assignment and thus the conclusions established for $T_H$ hold for $T_S^{(1)}$. For part 3) and 4), we have $T_S^{(1)} \xrightarrow{a.s.} Z$ by applying (8) directly. □

*Proof of Theorem 2.5.* Note that the map $g$ is a bijection and the corresponding inverse map is $g^{-1} : \mathbb{R}^p \to \mathbb{R}^p, g^{-1}(x) = \tau^{-1}x - \Delta_1$. According to the definitions of $g$ and $h$, we can represent $r(Y)$ in (10) as $r(Y) = h(Z) \cdot \mathbb{1}(s_1 = 1) + h(g^{-1}(Z)) \cdot \mathbb{1}(s_2 = 1)$. Furthermore, the result in (11) gives that $T_H = Z \cdot \mathbb{1}(\widetilde{s}_1 = s_1) + g^{-1}(Z) \cdot \mathbb{1}(\widetilde{s}_1 > s_1) + g(Z) \cdot \mathbb{1}(\widetilde{s}_1 < s_1)$.

If $s_1 = 1$, the event $\{\widetilde{s}_1 = 1\} = \{r(Y) > \pi_0\} = \{h(Z) > \pi_0\} = \{Z : Z \in R_3^c\}$ with probability 1. Consequently, we have

$$\begin{aligned} P(a^T T_H \leq t | s_1 = 1) &= P(a^T T_H \leq t, \widetilde{s}_1 = 1 | s_1 = 1) + P(a^T T_H \leq t, \widetilde{s}_2 = 1 | s_1 = 1) \\ &= P(a^T Z \leq t, \widetilde{s}_1 = 1 | s_1 = 1) + P(a^T g(Z) \leq t, \widetilde{s}_2 = 1 | s_1 = 1) \\ &= P(a^T Z \leq t, Z \in R_3^c | s_1 = 1) + P(a^T g(Z) \leq t, Z \in R_3 | s_1 = 1). \end{aligned}$$

Since $Z$ and $s_1$ are independent, it follows that

$$P(a^T T_H \leq t | s_1 = 1) = P(a^T Z \leq t, Z \in R_3^c) + P(a^T g(Z) \leq t, Z \in R_3),$$

which is $\Phi_p(R_2 \cap R_3^c) + \Phi_p(g^{-1}(R_2) \cap R_3)$. Because $Z$ is multivariate standard normal and $a$ has unit Euclidean norm, the random variable $a^T Z$ is thus standard normal. Therefore, we have $\Phi(t) = P(a^T Z < t) = \Phi_p(R_2)$, yielding that

$$P(a^T T_H \leq t | s_1 = 1) - \Phi(t) = \Phi_p(g^{-1}(R_2) \cap R_3) - \Phi_p(R_2 \cap R_3).$$

Following the same argument, if $s_2 = 1$, the event $\{\widetilde{s}_1 = 1\} = \{Z : h(g^{-1}(Z)) > \pi_0\} = \{Z : Z \in g(R_3^c)\}$ with probability 1, and thus we have

$$\begin{aligned}
P(a^T T_H \le t | s_2 = 1) &= P(a^T T_H \le t, \widetilde{s}_1 = 1 | s_2 = 1) + P(a^T T_H \le t, \widetilde{s}_2 = 1 | s_2 = 1) \\
&= P(a^T g^{-1}(Z) \le t, Z \in g(R_3^c)) + P(a^T Z \le t, Z \in g(R_3)) \\
&= \Phi_p(g(R_2) \cap g(R_3^c)) + \Phi_p(R_2 \cap g(R_3)),
\end{aligned}$$

where the property of $g(R_3^c) = g(R_3)^c$ is used. We thus have $P(a^T T_H \le t | s_2 = 1) - \Phi(t) = \Phi_p(g(R_2) \cap g(R_3^c)) - \Phi_p(R_2 \cap g(R_3^c))$. Consequently, $P(a^T T_H \le t) - \Phi(t)$ is equal to

$$\begin{aligned}
&[P(a^T T_H \le t | s_1 = 1) - \Phi(t)]P(s_1 = 1) + [P(a^T T_H \le t | s_2 = 1) - \Phi(t)]P(s_2 = 1) \\
&= \pi_1[\Phi_p(g^{-1}(R_2) \cap R_3) - \Phi_p(R_2 \cap R_3)] + \pi_2[\Phi_p(g(R_2) \cap g(R_3^c)) - \Phi_p(R_2 \cap g(R_3^c))],
\end{aligned}$$

which concludes the proof. □

*Proof of Lemma 2.6.* When $\tau > 1$, we have $h(x) - \pi_0 = (\tau^2 - 1)\left(x + \frac{\tau\Delta_2}{\tau^2-1}\right)^2 - \frac{c_0}{\tau^2-1}$, according to the definition of $h$ and $c_0$.

If $c_0 > 0$, it is easy to check that $(a_\pm(\theta))$ in (12a) are the the two roots of the equation $h(x) = \pi_0$. Therefore, the set $R_3 = \{h(x) < \pi_0\} = (a_-(\theta), a_+(\theta))$. If $c_0 \le 0$, we have $\tau > 1$ because otherwise $\tau = 1$ and $\Delta_2 = 0$, which leads to $\theta \in \Theta_0$. In this case, the set $R_3 = \varnothing$, which is $(a_-(\theta), a_+(\theta))$ since $a_-(\theta)$ is equal to $a_+(\theta)$.

If $c_0 > 0$ and $\tau = 1$, the quadratic equation $h(x) - \pi_0 = 0$ degenerates to a linear equation. Specifically, we have $h(x) - \pi_0 = 2\Delta_2 x + \Delta_2^2 - \pi_0$. Therefore, we have $R_3 = (\pi_0/(2\Delta_2) - \Delta_2/2, +\infty)$ if $\Delta_2 > 0$, and $R_3 = (-\infty, \pi_0/(2\Delta_2) - \Delta_2/2)$ if $\Delta_2 < 0$. □

*Proof of Theorem 2.8.* For the univariate case when $p = 1$, the set $R_2$ in Theorem 2.5 is $(-\infty, t)$ since the contrast coefficient $a$ is 1. For any $a \le b \in \bar{\mathbb{R}}$, we define

$$\begin{aligned}
A(t, a, b) &= (-\infty, t) \cap ((-\infty, a) \cup (b, +\infty)) = (-\infty, t \wedge a) \cup (b, t \vee b) \\
B(t, a, b) &= (-\infty, t) \cap (a, b) = (a, a \vee (t \wedge b)),
\end{aligned}$$

which leads to

$$\Phi(A(t, a, b)) = \Phi(t \wedge a) + \Phi(t \vee b) - \Phi(b); \quad \Phi(B(t, a, b)) = \Phi(a \vee (t \wedge b)) - \Phi(a).$$

According to Lemma 2.6, we have the set $R_3 = (a_-, a_+)$. It follows that $A(t, a_-, a_+) = R_2 \cap R_3^c$ and $B(t, a_-, a_+) = R_2 \cap R_3$. Let $b_- = g(a_-) = \tau a_- + \Delta_2$ and $b_+ = g(a_+)\tau a_+ + \Delta_2$. By applying Theorem 2.5, we obtain that

$$\begin{aligned}
P(T \le t) - \Phi(t) &= \pi_1[\Phi(B(t/\tau - \Delta_1, a_-, a_+)) - \Phi(B(t, a_-, a_+))] \\
&\quad + \pi_2[\Phi(A(\tau t + \Delta_2, b_-, b_+)) - \Phi(A(t, b_-, b_+))] \\
&= \pi_1[\Phi((b_- \vee (t \wedge b_+))/\tau - \Delta_1) - \Phi(a_- \vee (t \wedge a_+))] \\
&\quad + \pi_2[\Phi(\tau(t \wedge a_-) + \Delta_2) + \Phi(\tau(t \vee a_+) + \Delta_2) - \Phi(t \wedge b_-) - \Phi(t \vee b_+)],
\end{aligned}$$

which leads to the result in (13). □

*Proof of Lemma 2.9.* We denote $T$ in (8) as $T = g_1(Z, \Delta_1, \tau, \pi_0)s_1 + g_2(Z, \Delta_1, \tau, \pi_0)s_2$ to emphasize its dependency on $(Z, \Delta_1, \tau, \pi_0)$. Recall that $Z$ is independent with $(s_1, s_2)$, therefore we have the conditional random variable $T|(s_1 = 1) = g_1(Z, \Delta_1, \tau, \pi_0)$. For both hard and soft assignments, $\widetilde{s}_1, \widetilde{s}_2$ is a function of $r(Y) - \pi_0$, and $r(Y)|(s_1 = 1) = (\tau Z + \tau\Delta_1)^T(\tau Z + \tau\Delta_1) - Z^T Z$. Therefore, it is easy to see that $g_1(Z, \Delta_1, \tau, \pi_0) = -g_1(-Z, -\Delta_1, \tau, \pi_0)$. Since $Z$ and $-Z$ are identically distributed, we will have the same distribution for $|a^T T||(s_1 = 1)$ when we change $\Delta_1$ to $|\Delta_1|$. Similarly, the distribution of $|a^T T||(s_2 = 1)$ depends on $\Delta_1$ through the absolute values $|\Delta_1|$. Therefore, the distribution of $|T|$ depends on $\Delta_1$ only through $|\Delta_1|$. This establishes the lemma. □

# B Comparison between RB-GMM and the multivariate $t$ mixtures method

In this section, we compare the robust Gaussian mixture models via the $M$ estimation in Section 3 with the multivariate $t$ mixtures method (Peel and McLachlan, 2000). We do not consider the spatial structure and focus on comparing the performance of these two approaches in terms of robustness. We replace the $M$ step in a traditional GMM by the robust $M$ step detailed in Section 3, termed as RB-GMM. The multivariate $t$ mixtures method is implemented in the `R` package `EMMIXuskew` (Lee and McLachlan, 2013), where the skewness parameters are set to be 0.

In the simulation, we simulate data using $K = 2$ clusters with the following parameter values

$$\mu_1 = \begin{pmatrix} 0 \\ 3 \end{pmatrix}, \quad \mu_2 = \begin{pmatrix} 3 \\ 0 \end{pmatrix}, \quad \Sigma_1 = \Sigma_2 = \begin{pmatrix} 1 & 0 \\ 0 & 1 \end{pmatrix}, \quad \pi_1 = 0.6, \quad \pi_2 = 0.4.$$

We generate $n = 100$ observations and 5% of them are outliers independently drawn from $N(15, 1)$. We implemented the Gaussian mixture model (GMM), the proposed robust GMM without spatial structures (RB-GMM), and the multivariate $t$ mixtures method (MIX$t$). The table below reports the relative errors of each estimated parameter using the Euclidean norm for both the mean and $\pi$, and the 2-norm for the covariance matrices, averaged over 100 replications. The standard errors are reported in parenthesis.

| Method | $\mu_1$ | $\mu_2$ | $\Sigma_1$ | $\Sigma_2$ | $\pi$ |
|---|---|---|---|---|---|
| GMM | 0.69 (0.11) | 5.07 (0.24) | 5.42 (1.31) | 9.29 (1.62) | 0.59 (0.03) |
| RB-GMM ($q = 70\%$) | 0.07 (0.00) | 0.12 (0.01) | 0.45 (0.01) | 0.68 (0.05) | 0.11 (0.02) |
| RB-GMM ($q = 80\%$) | 0.08 (0.00) | 0.13 (0.01) | 0.45 (0.02) | 0.89 (0.06) | 0.09 (0.01) |
| RB-GMM ($q = 90\%$) | 0.11 (0.01) | 0.60 (0.16) | 0.73 (0.08) | 1.87 (0.19) | 0.13 (0.02) |
| MIX$t$ | 0.09 (0.01) | 0.24 (0.09) | 0.61 (0.08) | 0.85 (0.15) | 0.16 (0.02) |

We can see that both RB-GMM and MIX$t$ improve the estimation much compared to GMM. In addition, RB-GMM at $q = 70\%$ or 80% outperforms MIX$t$, but not so when $q = 90\%$. This suggests that if we tend to be conservative and use lower $q$ (thus presume there are more outliers than needed), RB-GMM leads to much better estimation performance

at least under this simulation setting. Therefore, the approach of RB-GMM provides flexibility to incorporate prior knowledge about the proportion of outliers. In our brain imaging applications, the proportion of brain volume occupied by tumors is usually small (often less than 1%), thus we recommended to use $q = 99\%$ as the default threshold. The comparison between RB-GMM and MIX$t$ is expected to depend on the settings, such as the deviation of the outliers from the two clusters. We observed that, compared to GMM and RB-GMM, the MIX$t$ approach takes much longer to run, as the number of degrees of freedoms requires extra computation at each iteration of the EM algorithm. MIX$t$ also seems more sensitive to the initial values of parameters. In fact, in this simulation we provided the true parameters as the initial values, mainly motivated by favoring MIX$t$ and make it work, but benefiting all the three approaches in comparison.

One of the major contribution of this paper is to combine spatial structures of $\pi$ with the robust EM procedure, which is tailored to the main application of biomedical imaging where template maps are indeed available and lesions often exist. We are not aware of whether the MIX$t$ method has been generalized to this spatial setting. This may be viewed as a future research topic.

# C Additional simulations comparing tumor size and shape

In this section, we conduct simulations following the settings in Section 4.2 but vary the tumor size and shape. We consider three additional scenarios and plot the background adjustment effects and bivariate density contours (similar to Figures 10 and 11): circular lesion with radius 6 in Figure 14, circular lesion with radius 3 in Figure 15, and a lesion formed as a union of two ellipses in Figure 16.

The performances of the proposed method are not affected by the lesion's smaller size or different shape. In all three figures, the first row shows a global non-homogeneous background change and little change in the lesion, but the adjusted observations and background difference in the second row are randomly distributed around zero and the lesion change is clearly visible. The last row of contour plots shows that RB-SGMM offers a standardized score close to normal and isolates the lesion successfully. The observation that the proposed method is not sensitive to lesion size or shape is explained by the fact that the treatment of outliers follows a voxelwise approach, so the lesion size or shape have little effect if the background parameters are estimated robustly. While the estimation of the background depends on spatial templates, the treatment of outliers does not. This allows the use of valuable spatial information for the background and yet being very flexible regarding the unknown location, size or shape of the lesion.

Figure 14: Simulated observations and background adjustment effects for Scenario B when the radius of the lesion is 6. The 1st row shows the simulated original scans and the corresponding contrast. The 2nd row shows the respective standardized images via background adjustment and their difference. The last row shows bivariate density contour plots of the observations with and without soft background adjustment within each class. The first column is for the original simulated observations, while the last three columns are the scores after background adjustment using the methods GMM, SGMM and RB-SGMM respectively.

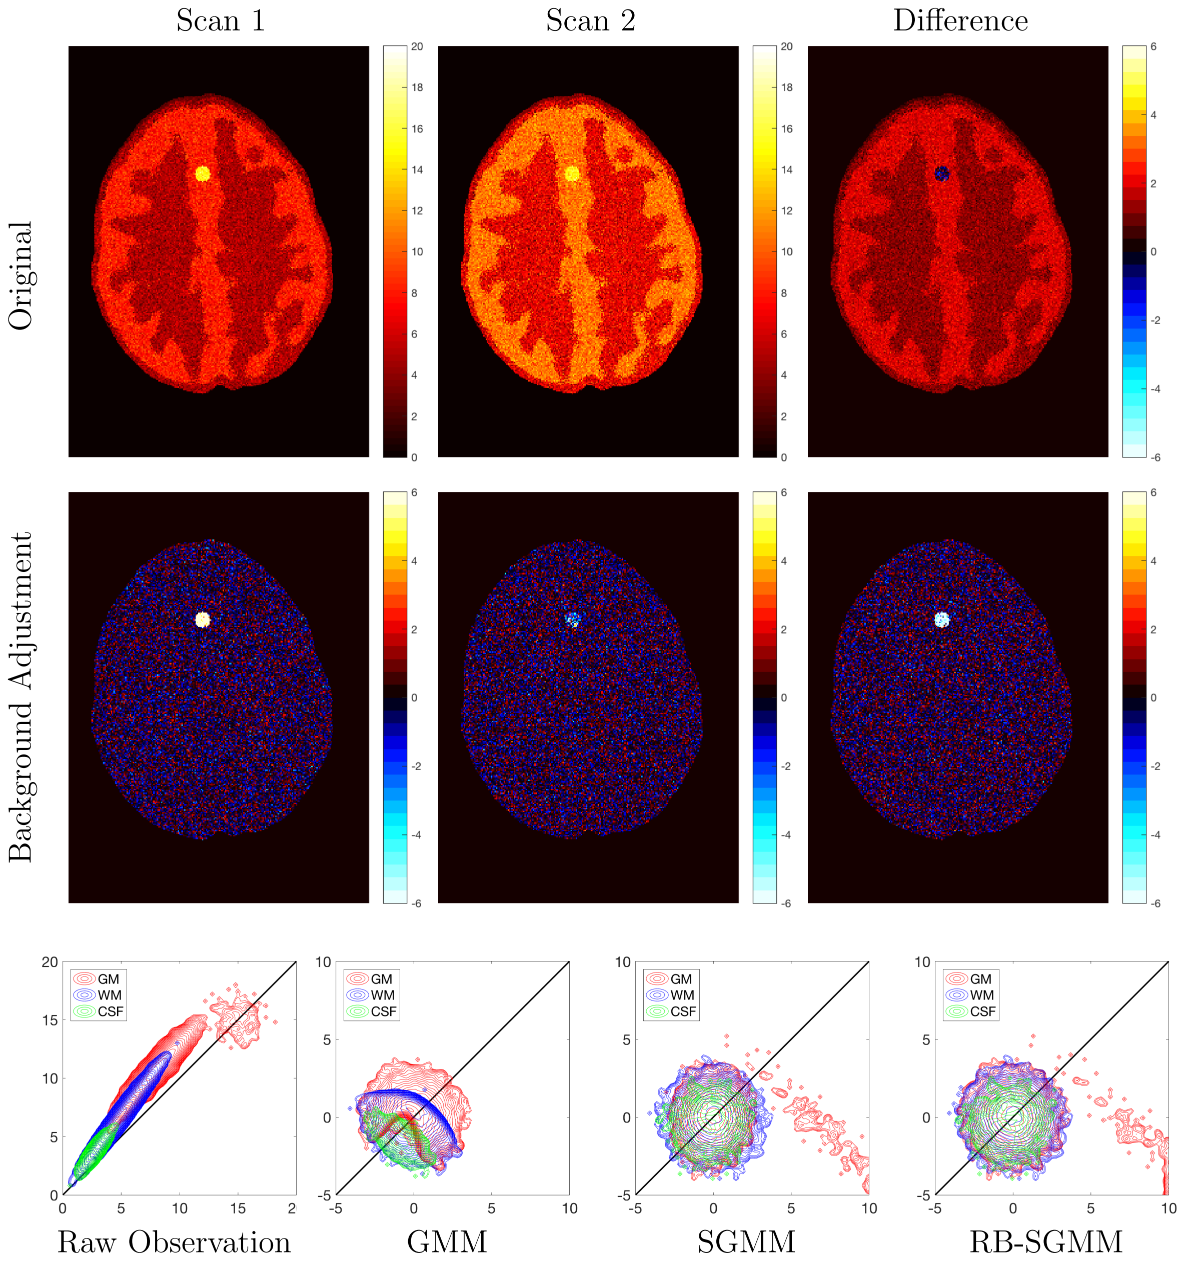

Figure 15: Simulated observations and background adjustment effects for Scenario B when the radius of the lesion is 3. The 1st row shows the simulated original scans and the corresponding contrast. The 2nd row shows the respective standardized images via background adjustment and their difference. The last row shows bivariate density contour plots of the observations with and without soft background adjustment within each class. The first column is for the original simulated observations, while the last three columns are the scores after background adjustment using the methods GMM, SGMM and RB-SGMM respectively.

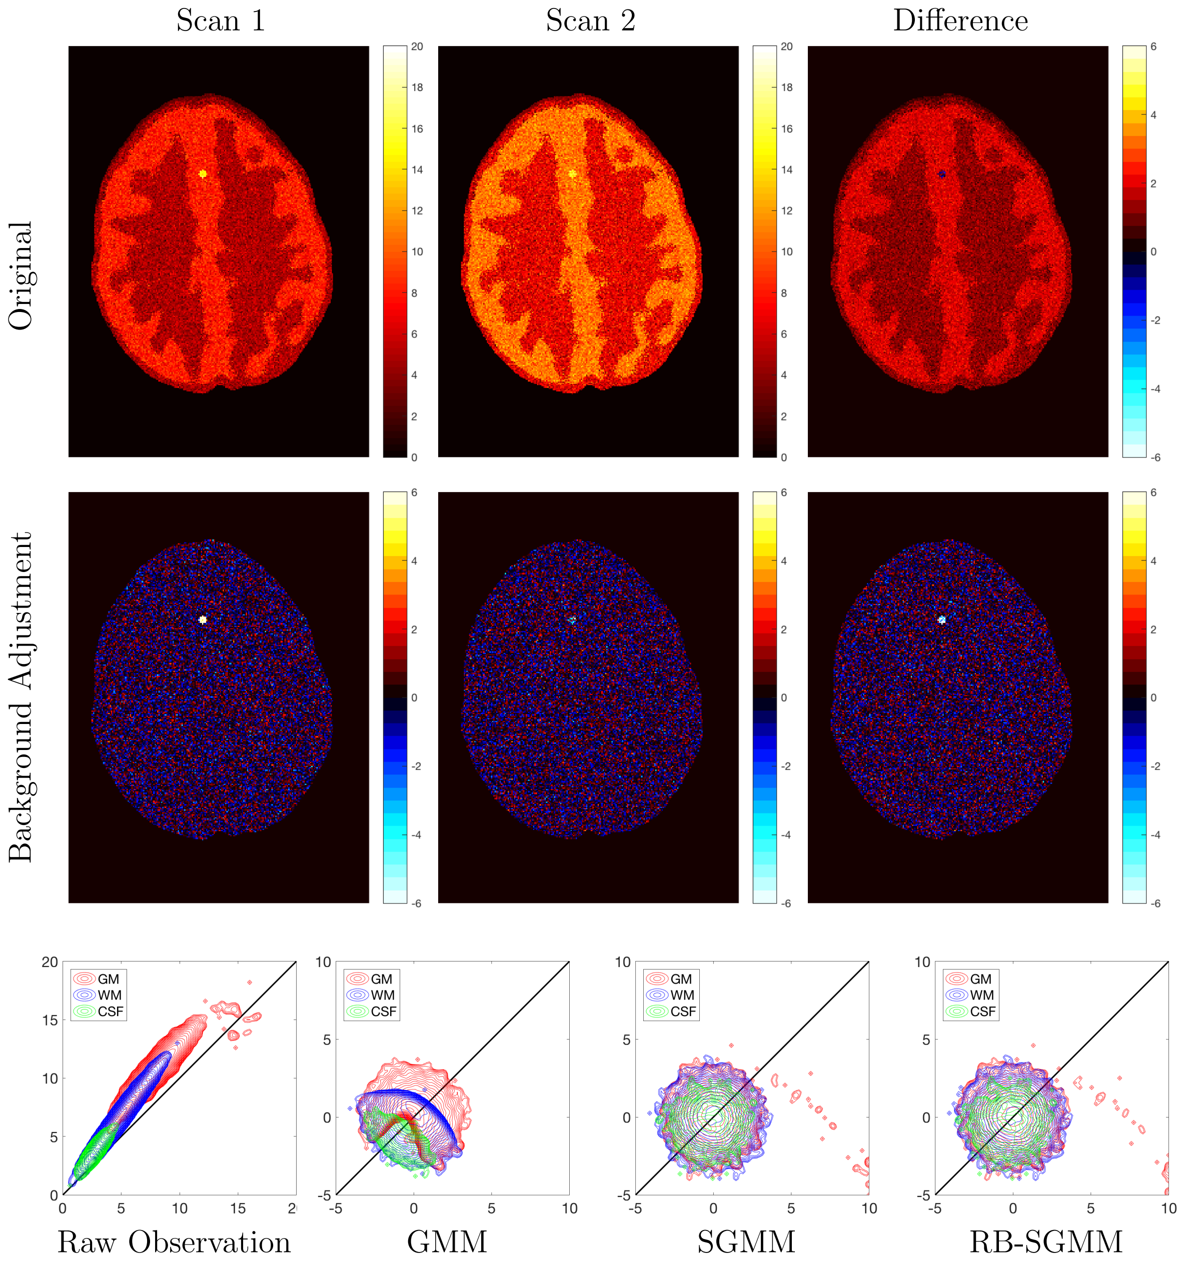

Figure 16: Simulated observations and background adjustment effects for Scenario B when the lesion is a union of two ellipses. The 1st row shows the simulated original scans and the corresponding contrast. The 2nd row shows the respective standardized images via background adjustment and their difference. The last row shows bivariate density contour plots of the observations with and without soft background adjustment within each class. The first column is for the original simulated observations, while the last three columns are the scores after background adjustment using the methods GMM, SGMM and RB-SGMM respectively.

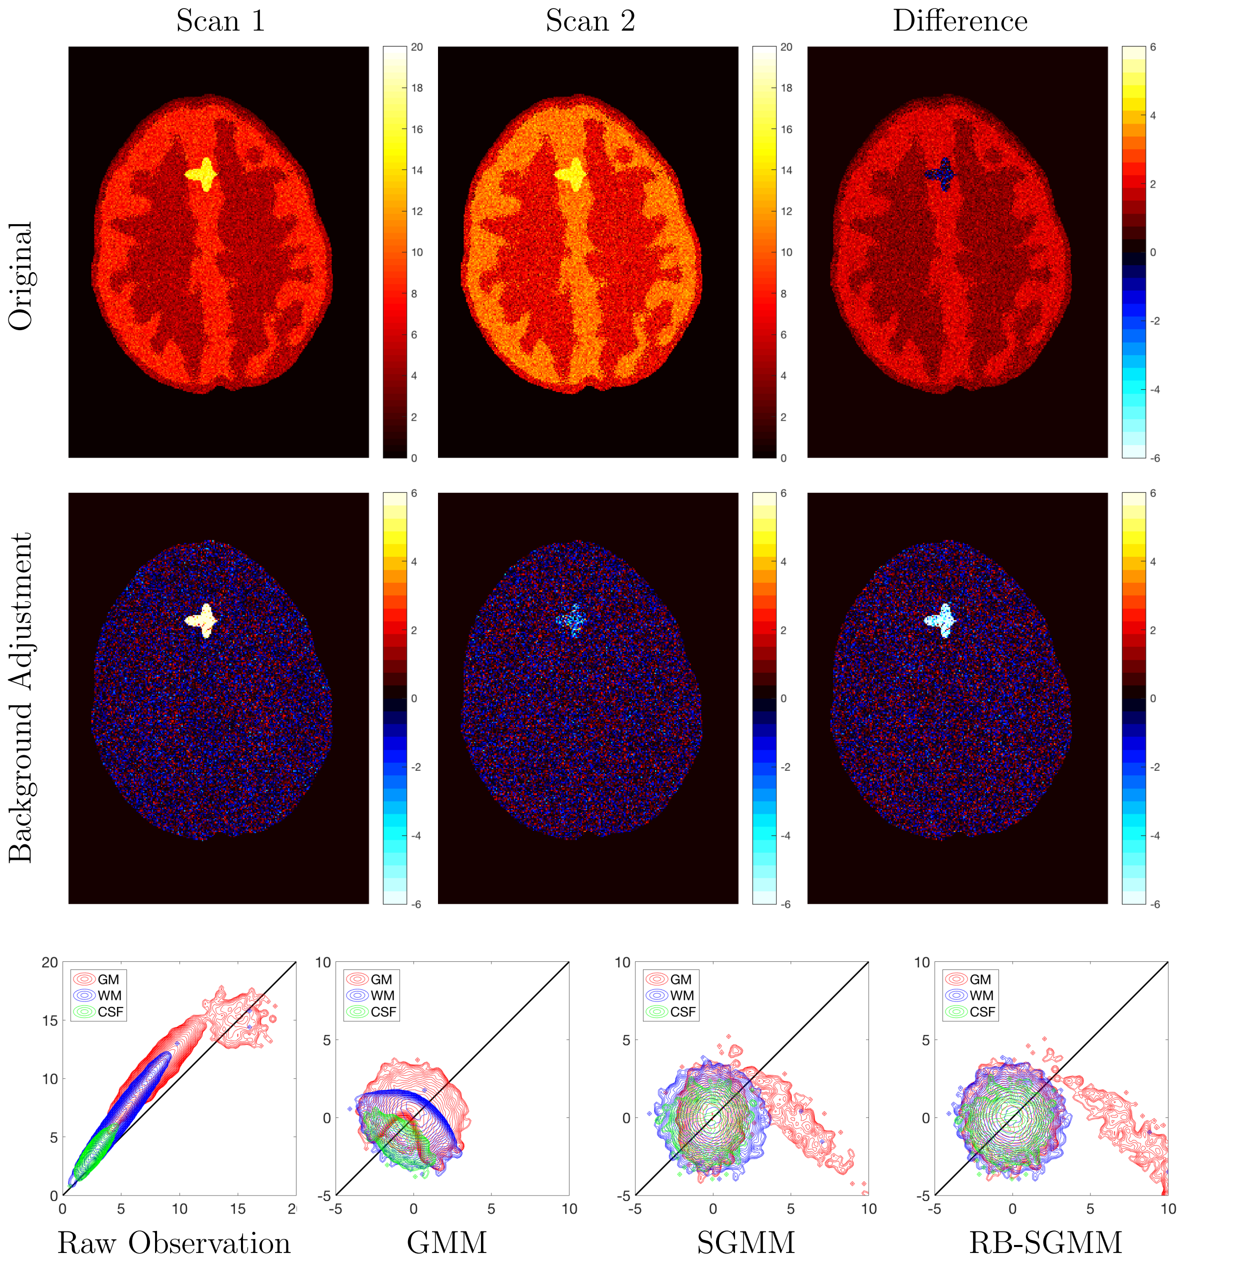

Supplement: Supplementary file 1 [file SGMM-supp.pdf]
